# Supplementary material for: Closing the Gap -- Formally Verifying Dynamically Typed Programs like Statically Typed Ones Using Hoare Logic -- Extended Version --
Source: arXiv:1501.02699 source file (2015-01-12)
Supplement: Supplementary file 1 [file app_type_hoare_logic.tex]

\todo{the algorithm is now flow-sensitive! Adapt rules accordingly!}

\vspace{0.1cm}
\noindent AXIOM: $\restricted$-CONST
\begin{center}
$\{\tau\} \Vnull \{\tau \wedge \llbracket \result \rrbracket \in \{\}\}$
\end{center}\todo{would null be permitted within brackets, this would be same as HL. neccessary?}

\noindent AXIOM: $\restricted$-VAR
\begin{center}
$\{\tau[\result := \PL{u}]\} \PL{u} \{\tau\}$ \hspace{1cm} where $\PL{u} \in \Var_L$.
\end{center}\todo{same as HL. neccessary?}

\noindent AXIOM: $\restricted$-IVAR

\begin{center}
$\{p\} @v \{p \wedge \llbracket \result \rrbracket \in \BaseTypeX\}$
\end{center}

where $p \rightarrow \llbracket \this.@v \rrbracket \in \BaseTypeX$, $\BaseTypeX \in 2^{\Class}$, $@v \in \Var_I$.

\noindent RULE: $\restricted$-ASGN - FLOW INSENSITIVE %(both normal and instance variables)
\begin{center}
\AxiomC{$\{p\} E \{p \wedge \llbracket \result \rrbracket \in \BaseTypeX\}$}
\RightLabel{with $v \in \Var_L$}
\UnaryInfC{$\{p\} v := E \{p \wedge \llbracket \result \rrbracket \in \BaseTypeX\}$}
\DisplayProof
\end{center}
where $p \equiv p' \wedge \llbracket v \rrbracket \in \BaseTypeX'$,
$v \not\in \free(p'), \BaseTypeX, \BaseTypeX' \in 2^{\Class}, \BaseTypeX \subseteq \BaseTypeX'$.

\noindent RULE: $\restricted$-IASGN - FLOW INSENSITIVE %(both normal and instance variables)
\begin{center}
\AxiomC{$\{p\} E \{p \wedge \llbracket \result \rrbracket \in \BaseTypeX\}$}
\RightLabel{with $@v \in \Var_I$}
\UnaryInfC{$\{p\} @v := E \{p \wedge \llbracket \result \rrbracket \in \BaseTypeX\}$}
\DisplayProof
\end{center}
where $p \equiv \TInv \wedge p'$,
$p' \rightarrow \llbracket this \rrbracket \in \{C\}$,
$@v \not\in \free(p'), \BaseTypeX \in 2^{\Class}$, $\BaseTypeX \subseteq \BaseTypeX_{C.@v}$.

\todo{use $\sqsubseteq$ instead of $\subseteq$ for types!!!}

\noindent RULE: $\restricted$-SEQ

\begin{center}
\AxiomC{$\{p\} S_1 \{r \wedge \llbracket \result \rrbracket \in \BaseTypeX_1\}$}
\AxiomC{$\{r\} S_2 \{q\}$}
\BinaryInfC{$\{p\} S_1; S_2 \{q\}$}
\DisplayProof
\end{center}

with $\BaseTypeX_1 \in 2^{\Class}$

\noindent RULE: $\restricted$-COND - PATH INSENSITIVE %(strong typesafe partial correctness)
%
% \begin{center}
% \AxiomC{$\begin{matrix}
%           \{p \wedge bool(B,true)\} S_1 \{q \wedge \llbracket result \rrbracket = T_1\} \\
%           \{p \wedge bool(B,false)\} S_2 \{q \wedge \llbracket result \rrbracket = T_2\}
%          \end{matrix}$}
%        
% \UnaryInfC{$\{p \wedge bool(B)\}$ if $B$ then $S_1$ else $S_2$ fi $\{q \wedge \llbracket result \rrbracket = T_1 \sqcup T_2\}$}
% \DisplayProof
% \end{center}
%
\begin{center}
\AxiomC{$\begin{matrix}
          \{p\} B \{p \wedge \llbracket \result \rrbracket \in \{bool\}\} \\
          \{p\} S_1 \{p \wedge \llbracket \result \rrbracket \in \BaseTypeX_1\} \\
          \{p\} S_2 \{p \wedge \llbracket \result \rrbracket \in \BaseTypeX_2\}
         \end{matrix}$}
       
\UnaryInfC{$\{p\}$ if $B$ then $S_1$ else $S_2$ fi $\{p \wedge \llbracket \result \rrbracket \in \BaseTypeX\}$}
\DisplayProof
\end{center}
where $\BaseTypeX_1 \subseteq \BaseTypeX, \BaseTypeX_2 \subseteq \BaseTypeX, \BaseTypeX,\BaseTypeX_1,\BaseTypeX_2 \in 2^{\Class}$.

\noindent RULE: $\restricted$-LOOP
\begin{center}
\AxiomC{$\begin{matrix}
          \{p\} B \{p \wedge \llbracket \result \rrbracket \in \{bool\} \} \\
          \{p\} S \{p \wedge \llbracket \result \rrbracket \in \BaseTypeX\}
         \end{matrix}$}
\UnaryInfC{$\{p\}$ while $B$ do $S$ od $\{p \wedge \llbracket \result \rrbracket \in \{\}\}$}
\DisplayProof
\end{center}

where $\BaseTypeX \in 2^{\Class}$.

\noindent RULE: $\restricted$-BLCK
\begin{center}
\AxiomC{$\{p\} S \{p \wedge \llbracket \result \rrbracket \in \BaseTypeX\}$}
%\RightLabel{ where $\result \not\in \{\Vector{x}\}$}
\UnaryInfC{$\{p'\}$ begin local $\Vector{u} := \Vector{t}; S \text{ end} \{\TInv \wedge \llbracket \result \rrbracket \in \BaseTypeX\}$}
\DisplayProof
\end{center}
where $p' \rightarrow p[\Vector{u}\Vector{\overline{u}} := \Vector{t}\Vector{\PL{null}}]$, $\{\Vector{u}\} \subseteq \Var_L \setminus \{\result\}$ and $\{\Vector{t}\} \subseteq \Var_L \cup \{\PL{null}\}$.

% \noindent RULE: $\restricted$-PASGN
% 
% \begin{center}
% $\{p[x_1,...,x_n := t_1,...,t_n] \wedge \llbracket t_n \rrbracket \in \BaseTypeX\} x_1,...,x_n := t_1,...,t_n \{p \wedge \llbracket \result \rrbracket \in \BaseTypeX\}$
% \end{center}

\noindent RULE: $\restricted$-METH
\begin{center}
\AxiomC{$\begin{matrix}
          \{p\} E_i \{p \wedge \llbracket \result \rrbracket \in \BaseTypeX_i \} \text{ for } i \in \mathbb{N}_n \\
          \{p_j\} l_0.m(l_1,...,l_n) \{\TInv \wedge \llbracket \result \rrbracket \in \BaseTypeX'_j\} \text{ for } j \in \mathbb{N}^1_k
         \end{matrix}$}
       
\UnaryInfC{$\{p\} E_0.m(E_1,...,E_n) \{p \wedge \llbracket \result \rrbracket \in \BaseTypeX\}$}
\DisplayProof
\end{center}
\todo{these are union types, not basetypes!!! (do not use $\BaseTypeX$, but $\UnionTypeX$)}
where $\BaseTypeX_0 = \{C_1,...,C_k\}$,
$p_j \equiv \TInv \wedge \llbracket l_0 \rrbracket \in \{C_j\} \wedge \bigwedge\limits_{i = 1}^n \llbracket l_i \rrbracket \in \BaseTypeX_{ij}$,
$p \wedge \llbracket l_0 \rrbracket \in \{C_j\} \rightarrow p_j$,
$\BaseTypeX'_j \subseteq \BaseTypeX$ and $\BaseTypeX_i \subseteq \BaseTypeX_{ij}$ for $i \in \mathbb{N}^1_n, j \in \mathbb{N}^1_k$.

\noindent RULE: $\restricted$-REC
\begin{center}
\AxiomC{$\begin{matrix}
          A \vdash \{p\} S \{q\}, \\
          A \vdash \{p_i\} \text{begin local }\this, \Vector{u_i} := l_i,\Vector{v_i}; S_i \text{ end} \{q_i\}, i \in \mathbb{N}^1_n \\
          p_i \rightarrow \llbracket l_i \rrbracket \in \{C_i\}, i \in \mathbb{N}^1_n
         \end{matrix}$}
       
\UnaryInfC{$\{p\} S \{q\}$}
\DisplayProof
\end{center}
where method $m_i(\Vector{u_i}) \{ S_i \} \in \Method_{C_i}$ for $i \in \mathbb{N}^1_n$ and $A \equiv \{p_1\} l_1.m_1(\Vector{v_1}) \{q_1\}, ..., \{p_n\} l_n.m_n(\Vector{v_n}) \{q_n\}$.

\noindent AXIOM: $\restricted$-NEW
\begin{center}
$\{p\} \mathbf{new}_C \{p \wedge \llbracket \result \rrbracket \in \{C\}\}$
\end{center}

\subsection{Soundness}

The rules given can be composed from the rules for typesafe partial correctness of \textbf{dyn} programs.

%\noindent :
\begin{proof}[RULE $\restricted$-ASGN]\hspace{0.1cm}\newline
 \begin{center}
  \AxiomC{$\{p\} E \{ p \wedge \llbracket \result \rrbracket \in \BaseTypeX \}$}
  \RightLabel{\scriptsize(CONS)}
  \UnaryInfC{$\{p\} E \{ p' \wedge \llbracket \result \rrbracket \in \BaseTypeX' \wedge \llbracket \result \rrbracket \in \BaseTypeX \}$}
  \RightLabel{\scriptsize(ASGN)}
  \UnaryInfC{$\{p\} v := E \{ p' \wedge \llbracket v \rrbracket \in \BaseTypeX' \wedge \llbracket \result \rrbracket \in \BaseTypeX \}$}
  \RightLabel{\scriptsize(CONS)}
  \UnaryInfC{$\{p\} v := E \{ p \wedge \llbracket \result \rrbracket \in \BaseTypeX\}$}
  \DisplayProof
 \end{center}
 with $\BaseTypeX \subseteq \BaseTypeX'$, $p \equiv p' \wedge \llbracket v \rrbracket \in \BaseTypeX'$, $v \not\in \free(p')$
 \hfill$\Box$
\end{proof}

\begin{proof}[RULE $\restricted$-IASGN]\hspace{0.1cm}\newline
 \begin{center}
  \AxiomC{$\{p\} E \{ p \wedge \llbracket \result \rrbracket \in \BaseTypeX \}$}
  \RightLabel{\scriptsize(CONS)}
  \UnaryInfC{$\{p\} E \{ \TInv[this.@v := \result] \wedge p' \wedge \llbracket \result \rrbracket \in \BaseTypeX \}$}
  \RightLabel{\scriptsize(ASGN)}
  \UnaryInfC{$\{p\} @v := E \{ \TInv \wedge p' \wedge \llbracket \result \rrbracket \in \BaseTypeX \}$}
  \RightLabel{\scriptsize(CONS)}
  \UnaryInfC{$\{p\} @v := E \{ p \wedge \llbracket \result \rrbracket \in \BaseTypeX\}$}
  \DisplayProof
 \end{center}
 with $\BaseTypeX \subseteq \BaseTypeX_{C.@v}$, $p \equiv \TInv \wedge p'$, $@v \not\in \free(p')$, $p' \rightarrow \llbracket this \rrbracket \in \{C\}$, $p \rightarrow \llbracket this.@v \rrbracket \in \BaseTypeX_{C.@v}$.

 the upper application of the CONS-rule needs further explanation:
 $\TInv$ can we written as a universally quantified conjunction of statements of the following form
 \[ \llbracket o \rrbracket \in \{C'\} \rightarrow \llbracket o.@u \rrbracket \in \BaseTypeX_{C'.@u} \]
 Now we consider an application of the substitution $[this.@v := \result]$ to the above statement:
 Since assignments to $@\mathbf{c}$ are not allowed in programs, we can safely assume that $@v \not= @\mathbf{c}$
 and conclude $\llbracket o \rrbracket \in \{C'\}[this.@v := \result] \equiv \llbracket o \rrbracket \in \{C'\}$.
 The left-hand side of the implication is thus unaffected by the substitution. For the right-hand side we
 have to distinguish the following cases
\begin{itemize}
 \item $@u \not= @v$:
 \[ \llbracket o.@u \rrbracket \in \BaseTypeX_{C'.@u}[this.@v := \result] \equiv \llbracket o.@u \rrbracket \in \BaseTypeX_{C'.@u} \]
 \item $@u = @v$:
 \begin{align*}
  \llbracket o.@u \rrbracket & \in \BaseTypeX_{C'.@u}[this.@v := \result] \equiv \\
  & \text{if } o = this \text{ then } \llbracket \result \rrbracket \in \BaseTypeX_{C'.@v} \text{ else } \llbracket o.@u \rrbracket \in \BaseTypeX_{C'.@u} \text{ fi}
 \end{align*}
\end{itemize}
From the first case, we see that all cases with other instance variables than the one assigned to are
also unaffected by the substitution.
Furthermore, $\llbracket this \rrbracket \in \{C\}$ and $\llbracket o \rrbracket \in \{C'\}$ with
$C \not= C'$ imply $o \not= this$. Hence, for all cases where the type of $o$ does not coincide with the type
of $this$, the above conditional is equivalent to its false branch $\llbracket o.@u \rrbracket \in \BaseTypeX_{C'.@u}$ and
the statement is thus unaffected by the substitution.
Summarizing, the substitution introduces a conditional in exactly one case: the one dealing with
the instance variable $@v$ of class $C$. For this case, we substitute the conditional by an equivalent
logical formula and get
\begin{align*}
 \llbracket o \rrbracket \in \{C\} \rightarrow & o \not= this \rightarrow \llbracket o.@v \rrbracket \in \BaseTypeX_{C.@v} \wedge \\
 \llbracket o \rrbracket \in \{C\} \rightarrow & o = this \rightarrow \llbracket \result \rrbracket \in \BaseTypeX_{C.@v}.
\end{align*}
Since $o = this$ implies $\llbracket o \rrbracket \in \{C\}$, we can write the entire substitution as follows
\[ \TInv[this.@v := \result] \leftrightarrow \TInv' \wedge \forall o \quantsep o = this \rightarrow \llbracket \result \rrbracket \in \BaseTypeX_{C.@v} \]
where $\TInv'$ is equivalent to $\TInv$ except for an added $o \not= this \rightarrow$ in the case for $C.@v$.
In fact, we can further simplify this to
\[ \TInv[this.@v := \result] \leftrightarrow \TInv' \wedge \llbracket \result \rrbracket \in \BaseTypeX_{C.@v}. \]

and since $\TInv \rightarrow \TInv'$ and $\BaseTypeX \subseteq \BaseTypeX_{C.@v}$, we have $p \wedge \llbracket \result \rrbracket \in \BaseTypeX \rightarrow \TInv[this.@v := \result]$.
 \hfill$\Box$
\end{proof}

\todo{$\restricted$-NEW rule}

\begin{proof}[RULE: $\restricted$-METH]\hspace{0.1cm}\newline
 \todo{incorporate usage of $TInv$ to derive types for instance variables of the calee into this rule}
 \todo{proof again from HL with quantification over objects and object creation}
\begin{center}
% \AxiomC{$\begin{matrix}
%           \{p\} E_i \{p \wedge \llbracket \result \rrbracket \in \BaseTypeX_i \} \text{ for } i \in \mathbb{N}_n \\
%           \{p_j\} l.m(l_1,...,l_n) \{p_j \wedge \llbracket \result \rrbracket \in \BaseTypeX'_j\} \text{ for } j \in \mathbb{N}^1_k
%          \end{matrix}$}
       
\AxiomC{$\begin{matrix}
          \{p_i\} E_i \{p_{i+1}[l_i := \result] \} \text{ for } i \in \mathbb{N}_n & (1)\\
          \{p_{n+1}\} l_0.m(l_1,...,l_n) \{p \wedge \llbracket \result \rrbracket \in \BaseTypeX\} & (2)
         \end{matrix}$}
\RightLabel{\scriptsize(METH)}
\UnaryInfC{$\{p\} E_0.m(E_1,...,E_n) \{p \wedge \llbracket \result \rrbracket \in \BaseTypeX\}$}
\DisplayProof
\end{center}

where $p_i \equiv p \wedge \bigwedge\limits_{j = 0}^{i-1} \llbracket l_j \rrbracket \in \BaseTypeX_j$, $l_i \in \Var, l_i \not\in free(E_j) \cup change(E_j)$ for all $i,j \in \mathbb{N}_n$.

Using the fact that the $l_i$ are not modified by the $E_j$, $(1)$ can be derived from the premises of $\restricted$-METH by
\begin{center}
\AxiomC{$\{p\} E_i \{p \wedge \llbracket \result \rrbracket \in \BaseTypeX_i \} \text{ for } i \in \mathbb{N}_n$}
\RightLabel{\scriptsize(INV)$\times n+1$}
\UnaryInfC{$\{p_i\} E_i \{p_{i+1}[l_i := \result] \} \text{ for } i \in \mathbb{N}_n$ \hspace{0.2cm} $(1)$}
\DisplayProof
\end{center}

Assuming that $\BaseTypeX_0 = \{C_1,...,C_k\}$, $(2)$ can be split using the DISJ rule and then derived from the
other $k$ premises of the $\restricted$-METH rule as follows

\begin{center}
\AxiomC{$\{p'''_j\} l_0.m(l_1,...,l_n) \{\TInv \wedge \llbracket \result \rrbracket \in \BaseTypeX'_j\} \text{ for } j \in \mathbb{N}^1_k$}
\RightLabel{\scriptsize(INV)$\times k$}
\UnaryInfC{$\{p''_j\} l_0.m(l_1,...,l_n) \{p \wedge \llbracket \result \rrbracket \in \BaseTypeX'_j\} \text{ for } j \in \mathbb{N}^1_k$}
\RightLabel{\scriptsize(CONS)$\times k$}
\UnaryInfC{$\{p'_j\} l_0.m(l_1,...,l_n) \{p \wedge \llbracket \result \rrbracket \in \BaseTypeX\} \text{ for } j \in \mathbb{N}^1_k$}
\RightLabel{\scriptsize(DISJ)$\times k-1$}
\UnaryInfC{$\{p_{n+1}\} l_0.m(l_1,...,l_n) \{p \wedge \llbracket \result \rrbracket \in \BaseTypeX\}$ \hspace{0.2cm} $(2)$}
\DisplayProof
\end{center}

where $p'_j \equiv p \wedge \llbracket l_0 \rrbracket \in \{C_j\} \wedge \bigwedge\limits_{i=1}^n \llbracket l_i \rrbracket \in \BaseTypeX_i$,
$p''_j \equiv p \wedge \llbracket l_0 \rrbracket \in \{C_j\} \wedge \bigwedge\limits_{i=1}^n \llbracket l_i \rrbracket \in \BaseTypeX_{ij}$,
$p'''_j \equiv \TInv \wedge \llbracket l_0 \rrbracket \in \{C_j\} \wedge \bigwedge\limits_{i=1}^n \llbracket l_i \rrbracket \in \BaseTypeX_{ij}$ for $j \in \mathbb{N}^1_k$ and
for all $i \in \mathbb{N}_n, j \in \mathbb{N}^1_k: \BaseTypeX_i \subseteq \BaseTypeX_{ij}$ and $\BaseTypeX'_j \subseteq \BaseTypeX$.
The reason the INV rule can be applied like this is that $(\Var_L \setminus \{\result\}) \cap change(l_0.m(l_1,...,l_n)) = \emptyset$
and except for $\TInv$, the typing assertion $p$ can only contain references to local variables. \hfill $\Box$
\end{proof}

\todo{other rules}

% 
% \noindent RULE: $\restricted$-BLCK
% composed from BLCK, CONS, PASGN
